# Supplementary material for: First-principles calculation of the electronic and optical properties of Gd$_{2}$FeCrO$_{6}$ double perovskite: Effect of Hubbard U parameter
Source: arXiv:2111.01864 source file (2021-11-02)
Supplement: Supplementary file 1 [file appendix1.tex]

\section{Supplementary Material} \label{sec:appendix}
    Here the ESI will be included.
